# Supplementary material for: Efficient Parallel Self-Adjusting Computation
Source: arXiv:2105.06712 source file (2021-05-14)
Supplement: Supplementary file 1 [file framework-appendix.tex]

\section{Additional Primitives}\label{appendix:additional-primitives} For convenience, we also support an \algorithmicallocarray{} operation
and a corresponding \algorithmicreadarray{} operation for allocating and reading arrays of modifiables.
We omit the details since they function, in essence, the same as their non-array counterparts.
We also supply a \algorithmicreadblock{} primitive that does not take any modifiables as arguments but instead runs
a thunk that can read modifiables directly. All the reads are then dynamically linked to the thunk so if any of them change,
the thunk can be re-executed. This is more flexible than \algorithmicread{}, but comes at some extra cost for
keeping track of the reads within a block of code.
We also support a \mbox{\algorithmicparfor{}} primitive, which executes a given function over a range of values in
parallel. Although this could be implemented manually by the programmer with a tree of binary forks, we
can perform the operation more efficiently and conveniently by including it as a primitive, since the manual version would create an unnecessary $S$ node in between every pair of $P$ nodes.
